# Supplementary material for: VMAS: Video-to-Music Generation via Semantic Alignment in Web Music Videos
Source: arXiv:2409.07450 source file (2024-09-11)
Supplement: Supplementary file 1 [file human_eval.tex]

\begin{table}[t]
    \caption{
    \textbf{Human Evaluation.} The evaluation of alignment is reported through the win rate. It focuses on (1) the synchronization between video transitions and music beats (MV beats) and (2) the genre alignment between music and video (Genre).
    }
    \centering
\setlength{\tabcolsep}{6pt}
\resizebox{0.95\textwidth}{!}{
\begin{tabular}{lcccccc}
\toprule
\multirow{2}{*}{Human Eval.}& \multicolumn{2}{c}{Symbolic Music} & & \multicolumn{3}{c}{Waveform Music} \\
\cmidrule{2-3} \cmidrule{5-7}
& CMT& Video2Music & & VidMusicGen & Vid2MLDM  & GVM  \\
\midrule
MV Beats &20.5&8.3&&15.7&25.5& \bf30.0 \\
Genre   &10.0&7.5&&17.5&27.5&\bf37.5 \\
\bottomrule
\end{tabular}
\label{tab:human_supp}
}
\end{table}
